# Supplementary material for: A unified immersed finite element error analysis for one-dimensional interface problems
Source: arXiv:2306.10018 source file (2023-05-26)
Supplement: Supplementary file 1 [file appendix.tex]

\newpage

\section{Appendix 1: Bramble-Hilbert on non-interface elements}
Bramble Hilbert theorem is a result that can be used to prove the error bound on the Radau projection on non-interface elements. We hope to extend it to non-interface elements

\begin{theorem}[Bramble-Hilbert in 1D]
Let $\hat{I}=[0,1]$ and let $\hat{\Pi}$ be a bounded \textbf{sublinear} functional on $H^{m+1}(\hat{I})$. Assume that 

$$\hat{\Pi}(w)=0,\qquad \forall w\in \P^m(\hat{I}).$$
Then there is $c>0$ such that 

$$\left|\hat{\Pi}(v)\right|\le c \left|v\right|_{k+1,\hat{I}}$$
\end{theorem}

This theorem is a direct consequence of the following lemma 

\begin{lemma}
There is a constant $c>0$ such that for any $v\in H^{m+1}(\hat{I})$, there is $w\in \P^m(\hat{I})$ such that 
$$\norm{v-w}_{m+1,\hat{I}}\le c|v|_{m+1}.$$\label{lemma:Grossman_trick}
\end{lemma}

\begin{proof}
The authors in \cite{grossmann_numerical_2007} gave an semi-explicit construction of $w$, they chose $w$ to be the unique $m-$th degree polynomial that verifies 
$$\int_{\hat{I}} v^{(k)}(x)-w^{(k)}(x)\ dx=0,\qquad k=0,\dots, m$$
This leads to an upper triangular system of equations with unique solution. After that, they used Poincar\'e's inequality: 

$$\norm{v-w}_{m+1,\hat{I}}^2\le C\left[|v-w|_{m+1,\hat{I}}^2+ \left(\int_{\hat{I}}v^k(x)-w^{(k)}(x)\ dx\right)^2\right]=C|v|_{m+1,\hat{I}}^2.$$

\end{proof}

\section{Appendix 2: Radau projection on non-interface elements}
Let 
\begin{align*}{B}_k(\u,\v)&= \int_0^T \int_{x_k}^{x_{k+1}} \v(x)^TS\u_{t}(x,t)\ dx  - \int_{x_k}^{x_{k+1}} \v_{x}(x)^T SA \u(x,t)\ dx \\
&+\v^T(x_{k+1}^-)S\left(A^+\u(x_{k+1}^-)+A^{-}\u(x_{k+1}^+)\right)-\v^T(x_{k}^+)S\left(A^-\u_h(x_{k}^+)+A^{+}\u(x_{k}^-)\right)\ dt.\end{align*}

We can write $B_k(\u,\v)$ as 

$$B_k(\u,\v)= \int_{x_k}^{x_{k+1}} \v(x)^TS\u_{t}(x,t)\ dx  +\tilde{B}_k(\u,\v).$$

The main idea of Radau projection is that for a given $\u$, we seek $\Pi_h^m\u\in S^m(I_k)$ such that the following Radau orthogonality condition holds

\begin{equation}\boxed{\tilde{B}_k(\Pi_h^m\u-\u,\v_h)=0,\quad \forall \v_h\in S^m(I_k):=\P^m(I_k)^2.}
\label{eqn:Radau_ortho}
\end{equation}

Instead of enforcing these condition on $\u$ directly, we enforce them on $\w=R^{\color{red}-1}\u$, where $$A=R \Lambda R^{\color{red}-1},\qquad \Lambda= \begin{pmatrix}\lambda_1<0&0\\ 0&\lambda_2>0\end{pmatrix}. $$

We define $\tilde{\Pi}^m_h\w$ such that $\Pi^m_h\u=R\tilde{\Pi}^m_h\w$. The Radau orthogonality condition can be written as

$$\begin{cases}
\ds \left(\tilde{\Pi}_h^m \w\right)_1(x_{k})=w_1(x_k),\\ \\
\ds \left(\tilde{\Pi}_h^m \w\right)_2(x_{k+1})=w_2(x_{k+1}),\\ \\ 
\ds \int_{x_k}^{x_{k+1}} \v_{h,x}^T(x) SR\Lambda \left(\tilde{\Pi}_h^m \w- \w\right)(x)\ dx=0, \quad \forall \v_h\in S^m(I_k).
\end{cases}
$$

The last condition can be written as 

$$\ds \int_{x_k}^{x_{k+1}} \v_{h}^T(x)  \left(\tilde{\Pi}_h^m \w- \w\right)(x)\ dx =0, \quad \forall \v_h\in S^{\color{red}m-1}(I_k).
$$
 This can be decoupled as 
 
 $$\ds \int_{x_k}^{x_{k+1}} x^i  \left(\tilde{\Pi}_h^m \w- \w\right)_{j}(x)=0, \quad i=0,\dots,m-1,\quad j=1,2. 
$$

The existence/construction of $\tilde{\Pi}_h^m\w$ is straightforward: Project $w_j$ onto $\P^{m-1}(I_k)$ and then add to it a multiple of the Legendre polynomial $L_m$ on $I_k$. 

The operator $\Pi^m_h$ is polynomial preserving. Therefore

\begin{equation}\norm{\u-\Pi^m_h\u}_{L^2(I_k)}\le C h^{m+1} |\u|_{m+1,2,I_k}.\label{eqn:hom_Radau_error}\end{equation}
